# Supplementary material for: Text2QR: Harmonizing Aesthetic Customization and Scanning Robustness for Text-Guided QR Code Generation
Source: arXiv:2403.06452 source file (2024-03-13)
Supplement: Supplementary file 1 [file X_suppl.tex]

\clearpage
\setcounter{page}{1}
\maketitlesupplementary

\section{Rationale}
\label{sec:rationale}
Having the supplementary compiled together with the main paper means that:
\begin{itemize}
\item The supplementary can back-reference sections of the main paper, for example, we can refer to \cref{sec:intro};
\item The main paper can forward reference sub-sections within the supplementary explicitly (e.g. referring to a particular experiment); 
\item When submitted to arXiv, the supplementary will already included at the end of the paper.
\end{itemize}
To split the supplementary pages from the main paper, you can use \href{https://support.apple.com/en-ca/guide/preview/prvw11793/mac#:~:text=Delete%20a%20page%20from%20a,or%20choose%20Edit%20%3E%20Delete).}{Preview (on macOS)}, \href{https://www.adobe.com/acrobat/how-to/delete-pages-from-pdf.html#:~:text=Choose%20%E2%80%9CTools%E2%80%9D%20%3E%20%E2%80%9COrganize,or%20pages%20from%20the%20file.}{Adobe Acrobat} (on all OSs), as well as \href{https://superuser.com/questions/517986/is-it-possible-to-delete-some-pages-of-a-pdf-document}{command line tools}.

@String(PAMI = {IEEE Trans. Pattern Anal. Mach. Intell.})
@String(IJCV = {Int. J. Comput. Vis.})
@String(CVPR= {IEEE Conf. Comput. Vis. Pattern Recog.})
@String(ICCV= {Int. Conf. Comput. Vis.})
@String(ECCV= {Eur. Conf. Comput. Vis.})
@String(NIPS= {Adv. Neural Inform. Process. Syst.})
@String(ICPR = {Int. Conf. Pattern Recog.})
@String(BMVC= {Brit. Mach. Vis. Conf.})
@String(TOG= {ACM Trans. Graph.})
@String(TIP  = {IEEE Trans. Image Process.})
@String(TVCG  = {IEEE Trans. Vis. Comput. Graph.})
@String(TMM  = {IEEE Trans. Multimedia})
@String(ACMMM= {ACM Int. Conf. Multimedia})
@String(ICME = {Int. Conf. Multimedia and Expo})
@String(ICASSP=	{ICASSP})
@String(ICIP = {IEEE Int. Conf. Image Process.})
@String(ACCV  = {ACCV})
@String(ICLR = {Int. Conf. Learn. Represent.})
@String(IJCAI = {IJCAI})
@String(PR   = {Pattern Recognition})
@String(AAAI = {AAAI})
@String(CVPRW= {IEEE Conf. Comput. Vis. Pattern Recog. Worksh.})
@String(CSVT = {IEEE Trans. Circuit Syst. Video Technol.})

@String(SPL	= {IEEE Sign. Process. Letters})
@String(VR   = {Vis. Res.})
@String(JOV	 = {J. Vis.})
@String(TVC  = {The Vis. Comput.})
@String(JCST  = {J. Comput. Sci. Tech.})
@String(CGF  = {Comput. Graph. Forum})
@String(CVM = {Computational Visual Media})

@String(PAMI  = {IEEE TPAMI})
@String(IJCV  = {IJCV})
@String(CVPR  = {CVPR})
@String(ICCV  = {ICCV})
@String(ECCV  = {ECCV})
@String(NIPS  = {NeurIPS})
@String(ICPR  = {ICPR})
@String(BMVC  =	{BMVC})
@String(TOG   = {ACM TOG})
@String(TIP   = {IEEE TIP})
@String(TVCG  = {IEEE TVCG})
@String(TCSVT = {IEEE TCSVT})
@String(TMM   =	{IEEE TMM})
@String(ACMMM = {ACM MM})
@String(ICME  =	{ICME})
@String(ICASSP=	{ICASSP})
@String(ICIP  = {ICIP})
@String(ACCV  = {ACCV})
@String(ICLR  = {ICLR})
@String(IJCAI = {IJCAI})
@String(PR = {PR})
@String(AAAI = {AAAI})
@String(CVPRW= {CVPRW})
@String(CSVT = {IEEE TCSVT})

@misc{Authors14,
 author = {FirstName LastName},
 title = {The frobnicatable foo filter},
 note = {Face and Gesture submission ID 324. Supplied as supplemental material {\tt fg324.pdf}},
 year = 2014
}

@misc{Authors14b,
 author = {FirstName LastName},
 title = {Frobnication tutorial},
 note = {Supplied as supplemental material {\tt tr.pdf}},
 year = 2014
}

@article{Alpher02,
author = {FirstName Alpher},
title = {Frobnication},
journal = PAMI,
volume = 12,
number = 1,
pages = {234--778},
year = 2002
}

@article{Alpher03,
author = {FirstName Alpher and  FirstName Fotheringham-Smythe},
title = {Frobnication revisited},
journal = {Journal of Foo},
volume = 13,
number = 1,
pages = {234--778},
year = 2003
}

@article{Alpher04,
author = {FirstName Alpher and FirstName Fotheringham-Smythe and FirstName Gamow},
title = {Can a machine frobnicate?},
journal = {Journal of Foo},
volume = 14,
number = 1,
pages = {234--778},
year = 2004
}

@inproceedings{Alpher05,
author = {FirstName Alpher and FirstName Gamow},
title = {Can a computer frobnicate?},
booktitle = CVPR,
pages = {234--778},
year = 2005
}

@inproceedings{stegastamp,
title={Stegastamp: {I}nvisible {H}yperlinks in {P}hysical {P}hotographs},
author={Matthew Tancik and Ben Mildenhall and Ren Ng},
booktitle={Proceedings of the IEEE/CVF Conference on Computer Vision and Pattern Recognition (CVPR)},
pages={2117--2126},
year={2020}
}

@InProceedings{HiDDeN,
  author = {Jiren Zhu and Russell Kaplan and Justin Johnson and Fei-Fei Li},
  title = {Hi{DD}e{N}: {H}iding {D}ata with {D}eep {N}etworks},
  booktitle = {The European Conference on Computer Vision (ECCV)},
  year = {2018}
}

@inproceedings{wengrowski2019light,
  title={Light {F}ield {M}essaging with {D}eep {P}hotographic {S}teganography},
  author={Eric Wengrowski and Kristin Dana},
  booktitle={Proceedings of the IEEE/CVF Conference on Computer Vision and Pattern Recognition (CVPR)},
  pages={1515--1524},
  year={2019}
}

@article{SteGAN_review,
  title={Recent {A}dvances of {I}mage {S}teganography with {G}enerative {A}dversarial {N}etworks},
  author={Jia Liu and Yan Ke and Yu Lei and Zhuo Zhang and Jun Li and Peng Luo and Minqing Zhang and Xiaoyuan Yang},
  journal={arXiv preprint arXiv:1907.01886},
  year={2019}
}

@article{SGAN,
  title={Steganographic {G}enerative {A}dversarial {N}etworks},
  author={Denis Volkhonskiy and Ivan Nazarov and Evgeny Burnaev},
  journal={arXiv preprint arXiv:1703.05502 },
  year={2017}
}

@InProceedings{SSGAN,
  author={Haichao Shi and Jing Dong and Wei Wang and Yinlong Qian and Xiaoyu Zhang},
  title={SSGAN: {S}ecure {S}teganography {B}ased on {G}enerative {A}dversarial {N}etworks},
  booktitle={Advances in Multimedia Information Processing -- PCM 2017},
  year={2018},
  pages={534--544}
}

@InProceedings{GNCNN,
  author = {Yinlong Qian and Jing Dong and Wei Wang and Tieniu Tan},
  title = {Deep learning for steganalysis via convolutional neural networks},
  booktitle = {Media Watermarking, Security, and Forensics},
  volume={9409},
  pages = {171--180},
  year = {2015}
}

@article{ASDL-GAN,
  author={Weixuan Tang and Shunquan Tan and Bin Li and Jiwu Huang},
  journal={IEEE Signal Processing Letters},
  title={Automatic {S}teganographic {D}istortion {L}earning {U}sing a {G}enerative {A}dversarial {N}etwork},
  volume={24},
  number={10},
  year={2017},
  pages={1547--1551}
}

@article{UT-SCA-GAN,
  title={Spatial {I}mage {S}teganography {B}ased on {G}enerative {A}dversarial {N}etwork},
  author={Jianhua Yang and Kai Liu and Xiangui Kang and Edward K. Wong and Yun-Qing Shi},
  journal={arXiv preprint arXiv:1804.07939},
  year={2018}
}

@article{CNNAE,
  author={Weixuan Tang and Bin Li and Shunquan Tan and Mauro Barni and Jiwu Huang},
  journal={IEEE Transactions on Information Forensics and Security},
  title={C{NN}-{B}ased {A}dversarial {E}mbedding for {I}mage {S}teganography},
  year={2019},
  volume={14},
  number={8},
  pages={2074--2087}
}

@article{Hu,
  author={Donghui Hu and Liang Wang and Wenjie Jiang and Shuli Zheng and Bin Li},
  journal={IEEE Access},
  title={A {N}ovel {I}mage {S}teganography {M}ethod via {D}eep {C}onvolutional {G}enerative {A}dversarial {N}etworks},
  year={2018},
  volume={6},
  pages={38303--38314}
}

@article{Ke2019,
  author={Yan Ke and Min-qing Zhang and Jia Liu and Ting-ting Su and Xiao-yuan Yang},
  title={Generative steganography with {K}erckhoffs' principle},
  journal={Multimedia Tools and Applications},
  year={2019},
  volume={78},
  number={10},
  pages={13805--13818},
}

@article{SteganoGAN,
  title = {SteganoGAN: {H}igh {C}apacity {I}mage {S}teganography with {G}ANs},
  author = {Kevin Alex Zhang and Alfredo Cuesta-Infante and Lei Xu and Kalyan Veeramachaneni},
  journal={arXiv preprint arXiv:1901.03892},
  year={2019}
}

@article{Adversarial_Examples,
  title = {Synthesizing {R}obust {A}dversarial {E}xamples},
  author = {Anish Athalye and Logan Engstrom and Andrew Ilyas and Kevin Kwok},
  journal={arXiv preprint arXiv:1707.07397},
  year={2017}
}

@InProceedings{Physical_Attacks1,
  author = {Kevin Eykholt and Ivan Evtimov and Earlence Fernandes and Bo Li and Amir Rahmati and Chaowei Xiao and Atul Prakash and Tadayoshi Kohno and Dawn Song},
  title = {Robust {P}hysical-{W}orld {A}ttacks on {D}eep {L}earning {V}isual {C}lassification},
  booktitle = {Proceedings of the IEEE/CVF Conference on Computer Vision and Pattern Recognition (CVPR)},
  year = {2018}
}

@article{Physical_Attacks2,
  title = {Physical {A}dversarial {E}xamples for {O}bject {D}etectors},
  author = {Kevin Eykholt and Ivan Evtimov and Earlence Fernandes and Bo Li and Amir Rahmati and Florian Tramer and Atul Prakash and Tadayoshi Kohno and Dawn Song},
  journal = {arXiv preprint arXiv:1807.07769},
  year = {2018}
}

@article{Physical_Attacks3,
  title = {Adversarial examples in the physical world},
  author = {Alexey Kurakin and Ian Goodfellow and Samy Bengio},
  journal={arXiv preprint arXiv:1607.02533},
  year={2016},
}

@InProceedings{Physical_Attacks4,
  title={ShapeShifter: {R}obust {P}hysical {A}dversarial {A}ttack on {F}aster {R}-{CNN} {O}bject {D}etector},
  author={Shang-Tse Chen and Cory Cornelius and Jason Martin and Duen Horng (Polo) Chau},
  booktitle={Machine Learning and Knowledge Discovery in Databases},
  year={2019},
  pages={52--68},
  isbn={978-3-030-10925-7},
  publisher={Springer International Publishing},
}

@InProceedings{JPEG,
  author={Richard Shin and Dawn Song},
  title={JPEG-resistant {A}dversarial {I}mages},
  booktitle={NeurIPS Workshop on Machine Learning and Computer Security},
  year={2017}
}

@InProceedings{AAAI,
  author={Steve T.K. Jan and Joseph Messou and Yen-Chen Lin and Jia-Bin Huang and Gang Wang},
  title={Connecting the {D}igital and {P}hysical {W}orld: {I}mproving the {R}obustness of {A}dversarial {A}ttacks},
  booktitle={AAAI},
  year={2019}
}

@article{Image_Transformation,
  title = {Image {T}ransformation can make {N}eural {N}etworks more robust against {A}dversarial {E}xamples},
  author = {Dang Duy Thang and Toshihiro Matsui},
  journal={arXiv preprint arXiv:1901.03037},
  year={2019}
}

@InProceedings{Perceptual_Losses,
  author={Justin Johnson and Alexandre Alahi and Fei-Fei Li},
  title={Perceptual {L}osses for {R}eal-{T}ime {S}tyle {T}ransfer and {S}uper-{R}esolution},
  booktitle={The European Conference on Computer Vision (ECCV)},
  year={2016},
  pages={694--711}
}

@InProceedings{Perceptual_Similarity,
  title = {Generating {I}mages with {P}erceptual {S}imilarity {M}etrics based on {D}eep {N}etworks},
  author = {Alexey Dosovitskiy and Thomas Brox},
  booktitle = {Advances in Neural Information Processing Systems},
  pages = {658--666},
  year = {2016}
}

@InProceedings{LPIPS,
  author = {Richard Zhang and Phillip Isola and Alexei A. Efros and Eli Shechtman and Oliver Wang},
  title = {The {U}nreasonable {E}ffectiveness of {D}eep {F}eatures as a {P}erceptual {M}etric},
  booktitle = {Proceedings of the IEEE/CVF Conference on Computer Vision and Pattern Recognition (CVPR)},
  year = {2018}
}

@article{SSIM,
  author={Zhou Wang and Alan Conrad Bovik and Hamid Rahim Sheikh and Eero P. Simoncelli},
  journal={IEEE Transactions on Image Processing},
  title={Image quality assessment: from error visibility to structural similarity},
  year={2004},
  volume={13},
  number={4},
  pages={600--612}
}

@InProceedings{MSSIM,
  author={Zhou Wang and Eero P. Simoncelli and Alan Conrad Bovik},
  title={Multiscale structural similarity for image quality assessment},
  booktitle={The Thrity-Seventh Asilomar Conference on Signals, Systems Computers, 2003},
  year={2003},
  volume={2},
  pages={1398--1402}
}

@article{FSIM,
  author={Lin Zhang and Lei Zhang and Xuanqin Mou and David Zhang},
  journal={IEEE Transactions on Image Processing},
  title={F{SIM}: {A} {F}eature {S}imilarity {I}ndex for {I}mage {Q}uality {A}ssessment},
  year={2011},
  volume={20},
  number={8},
  pages={2378--2386}
}

@article{JND1,
  author={Yuting Jia and Weisi Lin and Ashraf A. Kassim },
  journal={IEEE Transactions on Circuits and Systems for Video Technology},
  title={Estimating {J}ust-{N}oticeable {D}istortion for {V}ideo},
  volume={16},
  number={7},
  year={2006},
  pages={820--829},
  doi={10.1109/TCSVT.2006.877397},
  month={July},
}

@article{JND2,
  author = {X.K. Yang and W.S. Ling and Z.K. Lu and E.P. Ong and S.S. Yao},
  title = {Just noticeable distortion model and its applications in video coding},
  journal = {Signal Processing: Image Communication},
  year = {2005},
  volume={20},
  Issue={7},
  pages = {662--680}
}

@article{JND3,
  author={Anmin Liu and Weisi Lin and Manoranjan Paul and Chenwei Deng and Fan Zhang},
  journal={IEEE Transactions on Circuits and Systems for Video Technology},
  title={Just {N}oticeable {D}ifference for {I}mages {W}ith {D}ecomposition {M}odel for {S}eparating {E}dge and {T}extured {R}egions},
  year={2010},
  volume={20},
  number={11},
  pages={1648--1652},
  month={Nov},
}

@article{JND4,
  author={Jinjian Wu and Guangming Shi and Weisi Lin and Anmin Liu and Fei Qi},
  journal={IEEE Transactions on Multimedia},
  title={Just {N}oticeable {D}ifference {E}stimation for {I}mages with {F}ree-{E}nergy {P}rinciple},
  year={2013},
  volume={15},
  number={7},
  pages={1705--1710},
  month={Nov},
}

@article{JND5,
  author={Jinjian Wu and Leida Li and Weisheng Dong and Guangming Shi and Weisi Lin and C.-C. Jay Kuo},
  journal={IEEE Transactions on Image Processing},
  title={Enhanced {J}ust {N}oticeable {D}ifference {M}odel for {I}mages with {P}attern {C}omplexity},
  year={2017},
  volume={26},
  number={6},
  pages={2682--2693},
  month={June},
}

@InProceedings{Lambertian,
  author={J. H. Lambert},
  booktitle={Photometria {S}ive de {M}ensure de {G}radibus {L}uminis, {C}olorum et {U}mbrae},
  year={1760},
}

@InProceedings{Lambertian_Reflectance,
  author={Sanjeev J. Koppal},
  title={Lambertian {R}eflectance},
  booktitle={Computer Vision: A Reference Guide},
  year={2014},
  pages={441--443},
  isbn={978-0-387-31439-6},
  doi={10.1007/978-0-387-31439-6_534},
}

@article{Phong,
  author = {B. T. Phong},
  journal = {Commun. ACM},
  number = {6},
  pages = {311--317},
  title = {Illumination for {C}omputer {G}enerated {P}ictures},
  year = {1975},
}

@InProceedings{TensorflowGraphicsIO2019,
   author = {Julien Valentin and Cem Keskin and Pavel Pidlypenskyi and Ameesh Makadia and Avneesh Sud and Sofien Bouaziz},
   title = {TensorFlow {G}raphics: {C}omputer {G}raphics {M}eets {D}eep {L}earning},
   year = {2019}
}

@InProceedings{Cameranoise,
  author = {Samuel W. Hasinoff},
  title = {Photon, {P}oisson {N}oise},
  booktitle = {Computer Vision: A Reference Guide},
  year={2014},
  pages={608--610},
  isbn={978-0-387-31439-6},
  doi={10.1007/978-0-387-31439-6_482},
}

@InProceedings{U-net,
  author={Olaf Ronneberger and Philipp Fischer and Thomas Brox},
  title={U-{N}et: {C}onvolutional {N}etworks for {B}iomedical {I}mage {S}egmentation},
  booktitle={Medical Image Computing and Computer-Assisted Intervention -- MICCAI 2015},
  year={2015},
  pages={234--241},
  isbn={978-3-319-24574-4},
}

@InProceedings{STN,
  title={Spatial {T}ransformer {N}etworks},
  author={Max Jaderberg and Karen Simonyan and Andrew Zisserman and koray kavukcuoglu},
  booktitle={Advances in Neural Information Processing Systems},
  pages = {2017--2025},
  year = {2015},
}

@InProceedings{Wasserstein,
  title={Wasserstein {G}enerative {A}dversarial {N}etworks},
  author={Martin Arjovsky and Soumith Chintala and L{\'e}on Bottou},
  booktitle={Proceedings of the 34th International Conference on Machine Learning},
  pages={214--223},
  year={2017},
}

@article{BCH,
   title = {On a {C}lass of {E}rror {C}orrecting {B}inary {G}roup {C}odes},
   author = {R.C. Bose and D.K. Ray-Chaudhuri},
   journal = {Information and Control},
   pages = {68--79},
   year = {1960},
}

@InProceedings{TPVM,
   author = {Zhongpai Gao and Guangtao Zhai and Chunjia Hu},
   title = {The {I}nvisible {QR} {C}ode},
   booktitle = {Proceedings of the 23rd ACM International Conference on Multimedia},
   year = {2015},
   pages = {1047--1050},
}

@inproceedings{morkel2005overview,
  title={An {O}verview of {I}mage {S}teganography.},
  author={Tayana Morkel and Jan HP Eloff and Martin S Olivier},
  booktitle={ISSA},
  volume={1},
  pages={2},
  year={2005}
}

@article{marvel1999spread,
  title={Spread {S}pectrum {I}mage {S}teganography},
  author={Lisa M Marvel and Charles G Boncelet and Charles T Retter},
  journal={IEEE Transactions on Image Processing},
  volume={8},
  number={8},
  pages={1075--1083},
  year={1999}
}

@article{johnson1998exploring,
  title={Exploring {S}teganography: {S}eeing the {U}nseen},
  author={Neil F Johnson and Sushil Jajodia},
  journal={Computer},
  volume={31},
  number={2},
  pages={26--34},
  year={1998}
}

@article{karybali2006efficient,
author={I. G. Karybali and K. Berberidis},
journal={IEEE Transactions on Information Forensics and Security},
title={Efficient {S}patial {I}mage {W}atermarking via {N}ew {P}erceptual {M}asking and {B}lind {D}etection {S}chemes},
year={2006},
volume={1},
number={2},
pages={256--274}
}

@article{mukherjee2004spatial,
author={D. P. Mukherjee and S. Maitra and S. T. Acton},
journal={IEEE Transactions on Multimedia},
title={Spatial {D}omain {D}igital {W}atermarking of {M}ultimedia {O}bjects for {B}uyer {A}uthentication},
year={2004},
volume={6},
number={1},
pages={1--15}
}

@article{tian2013ldft,
author={Huawei Tian and Yao Zhao and Rongrong Ni and Lunming Qin and Xuelong Li},
journal={IEEE Transactions on Cybernetics},
title={{LDFT}-{B}ased {W}atermarking {R}esilient to {L}ocal {D}esynchronization {A}ttacks},
year={2013},
volume={43},
number={6},
pages={2190--2201}
}

@article{chu2003dct,
author={W. C. Chu},
journal={IEEE Transactions on Multimedia},
title={{DCT}-based {I}mage {W}atermarking {U}sing {S}ubsampling},
year={2003},
volume={5},
number={1},
pages={34--38}
}

@inproceedings{luo2020distortion,
title={Distortion {A}gnostic {D}eep {W}atermarking},
author={Xiyang Luo and Ruohan Zhan and Huiwen Chang and Feng Yang and Peyman Milanfar},
booktitle={Proceedings of the IEEE/CVF Conference on Computer Vision and Pattern Recognition (CVPR)},
pages={13548--13557},
year={2020}
}

@article{zhang2019robust,
title={Robust {I}nvisible {V}ideo {W}atermarking with {A}ttention},
author={Kevin Alex Zhang and Lei Xu and Alfredo Cuesta-Infante and Kalyan Veeramachaneni},
journal={arXiv preprint arXiv:1909.01285},
year={2019}
}

@inproceedings{wengrowski2017reading,
title={Reading between the {P}ixels: {P}hotographic {S}teganography for {C}amera {D}isplay {M}essaging},
author={Eric Wengrowski and Kristin J Dana and Marco Gruteser and Narayan Mandayam},
booktitle={2017 IEEE International Conference on Computational Photography (ICCP)},
pages={1--11},
year={2017}
}

@article{RIHOOP,
author={Jun Jia and Zhongpai Gao and Kang Chen and Menghan Hu and Xiongkuo Min and Guangtao Zhai and Xiaokang Yang},
journal={IEEE Transactions on Cybernetics},
title={R{IHOOP}: {R}obust {I}nvisible {H}yperlinks in {O}ffline and {O}nline {P}hotographs},
year={2020},
pages={1-13}
}

@article{TERA,
author={Han Fang and Dongdong Chen and Feng Wang and Zehua Ma and Honggu Liu and Wenbo Zhou and Weiming Zhang and Neng-Hai Yu},
journal={IEEE Transactions on Multimedia}, 
title={T{ERA}: {S}creen-to-{C}amera {I}mage {C}ode with {T}ransparency, {E}fficiency, {R}obustness and {A}daptability}, 
year={2021},
pages={1-1}
}

@article{fang2018screen,
author={Han Fang and Weiming Zhang and Hang Zhou and Hao Cui and Nenghai Yu},
journal={IEEE Transactions on Information Forensics and Security},
title={Screen-{S}hooting {R}esilient {W}atermarking},
volume={14},
number={6},
pages={1403--1418},
year={2018}
}

@article{picode,
author={Changsheng Chen and Wenjian Huang and Baojian Zhou and Chenchen Liu and Wai Ho Mow},
journal={IEEE Transactions on Image Processing}, 
title={Pi{C}ode: {A} {N}ew {P}icture-{E}mbedding {2D} {B}arcode}, 
year={2016},
volume={25},
number={8},
pages={3444-3458}
}

@article{chen2018robust,
author={Changsheng Chen and Wenjian Huang and Lin Zhang and Wai Ho Mow},
journal={IEEE Transactions on Image Processing},
title={Robust and {U}nobtrusive {D}isplay-to-{C}amera {C}ommunications via {B}lue {C}hannel {E}mbedding},
volume={28},
number={1},
pages={156--169},
year={2018}
}

@article{racode,
author={Changsheng Chen and Baojian Zhou and Wai Ho Mow},
journal={IEEE Transactions on Circuits and Systems for Video Technology}, 
title={R{A} {C}ode: {A} {R}obust and {A}esthetic {C}ode for {R}esolution-{C}onstrained {A}pplications}, 
year={2018},
volume={28},
number={11},
pages={3300-3312}
}

@article{chu2013halftone, 
author={Hung-Kuo Chu and Chia-Sheng Chang and Ruen-Rone Lee and Niloy J Mitra},
title={Halftone {QR} {C}odes},
journal={ACM Transactions on Graphics (TOG)},
volume={32},
number={6},
pages={1--8},
year={2013}
}

@article{garateguy2014qr,
title={Q{R} {I}mages: {O}ptimized {I}mage {E}mbedding in {QR} {C}odes},
author={Gonzalo J Garateguy and Gonzalo R Arce and Daniel L Lau and Ofelia P Villarreal},
journal={IEEE Transactions on Image Processing},
volume={23},
number={7},
pages={2842--2853},
year={2014}
}

@article{imagenet,
  title={Imagenet {C}lassification with {D}eep {C}onvolutional {N}eural {N}etworks},
  author={Alex Krizhevskyand and Ilya Sutskever and Geoffrey E Hinton},
  journal={Advances in Neural Information Processing Systems},
  volume={25},
  pages={1097--1105},
  year={2012}
}

@inproceedings{hrnet,
title={Deep {H}igh-{R}esolution {R}epresentation {L}earning for {H}uman {P}ose {E}stimation},
author={Ke Sun and Bin Xiao and Dong Liu and Jingdong Wang},
booktitle={Proceedings of the IEEE/CVF Conference on Computer Vision and Pattern Recognition (CVPR)},
pages={5693--5703},
year={2019}
}

@article{SIFT,
title={Distinctive {I}mage {F}eatures from {S}cale-{I}nvariant {K}eypoints},
author={David G Lowe},
journal={International Journal of Computer Vision},
volume={60},
number={2},
pages={91--110},
year={2004}
}

@inproceedings{resnet,
title={Deep {R}esidual {L}earning for {I}mage {R}ecognition},
author={Kaiming He and Xiangyu Zhang and Shaoqing Ren and Jian Sun},
booktitle={Proceedings of the IEEE Conference on Computer Vision and Pattern Recognition (CVPR)},
pages={770--778},
year={2016}
}

@article{voc2012,
title={The {P}ascal {V}isual {O}bject {C}lasses {C}hallenge: {A} {R}etrospective},
author={Mark Everingham and SM Ali Eslami and Luc Van Gool and Christopher KI Williams and John Winn and Andrew Zisserman},
journal={International Journal of Computer Vision},
volume={111},
number={1},
pages={98--136},
year={2015}
}

@article{wang2020deep,
title={Deep {H}igh-{R}esolution {R}epresentation {L}earning for {V}isual {R}ecognition},
author={Jingdong Wang and Ke Sun and Tianheng Cheng and Borui Jiang and Chaorui Deng and Yang Zhao and Dong Liu and Yadong Mu and Mingkui Tan and Xinggang Wang and others},
journal={IEEE Transactions on Pattern Analysis and Machine Intelligence},
volume={43},
number={10},
pages={3349--3364},
year={2020}
}
