# Supplementary material for: Text2QR: Harmonizing Aesthetic Customization and Scanning Robustness for Text-Guided QR Code Generation
Source: arXiv:2403.06452 source file (2024-03-13)
Supplement: Supplementary file 2 [file Y_suppl.tex]

\clearpage
\setcounter{page}{1}
\maketitlesupplementary

\section{Limitation \& Future work}
Currently, our method exclusively accommodates Stable-Diffusion models with text-based prompts, rendering its application impractical for other image-to-image translation models. Moving forward, we aim to broaden the scope of our approach by evolving it into a versatile and customizable framework, which will facilitate seamless support for both text-to-image and image-to-image translation models.

\section{Additional Experiments}
\label{sec:selr}
\subsection{Visualization of intermediate results}
In Table~\ref{tab:comparison1}, we present the intermediate outcomes of Text2QR. Here, $I^{hc}$ represents the high-contrast grayscale input image, $M^r$ signifies the reorganized QR code, and $I^b$ denotes the synergistic blueprint image. Leveraging the information from $I^b$, we employ ControlNet to reconstruct the image $I^s$ and refine it through the SELR module to derive the aesthetically pleasing QR code $Q$. It is worth noting that $I^b$ preserves as much image content as possible under the premise of being scannable, which is critical for generating visually coherent output.
\subsection{Loss curve \& running time}

\begin{figure}[h]
    \centering
    \includegraphics[width=0.9\linewidth]{figs/curve.pdf}
    \caption{Curve of different metrics during SELR. We present metric curves for diverse samples, each represented by distinct colors. These curves illustrate metric variations over 400 iterations.}\label{fig:curve}
    \vspace{-5pt}
\end{figure}

In the SELR module, we enhance the scannability of $I^s$ by refining it through the update of its latent code. The loss function comprises a code loss $\mathcal{L}_{c}$ to regulate scanning robustness and a harmonizing loss $\mathcal{L}_{h}$ to augment visual quality. The synergy between these two losses facilitates swift convergence. Figure~\ref{fig:curve} illustrates the loss curve and two metrics, namely the PSNR (dB) between $I^s$ and $Q$, and the error level $e$ between $M^r$ and $Q$ for various samples represented by different colors.
It is noteworthy that, despite a default of 400 steps for sample updates, satisfactory results are attainable at intermediate steps. This expeditious convergence is attributed to our blueprint constraining the generated content to a significant extent, allowing SELR refinement to swiftly achieve an acceptable outcome. As the refinement process solely involves updating the latent code of $I^s$, computational efficiency is achieved. On an NVIDIA RTX 4090 GPU, the refinement converges within 60 seconds for 1024$\times$1024 images.

\subsection{Visualization of iteration}

\setlength{\myfigwidth}{0.22\linewidth} % Adjust the size as needed
\begin{table}[h]
    \caption{Visualization of iterative refinement.}
    \label{tab:selr}
    \centering
    \begin{tabularx}{\linewidth}{>{\centering\arraybackslash}X *{4}{>{\centering\arraybackslash}X}}

    \toprule
    input (un-scannable) & iter=100 & iter=200 & iter=400 (scannable) \\
    \midrule

    \includegraphics[width=\myfigwidth, height=\myfigwidth]{CVPR2024-T2QR/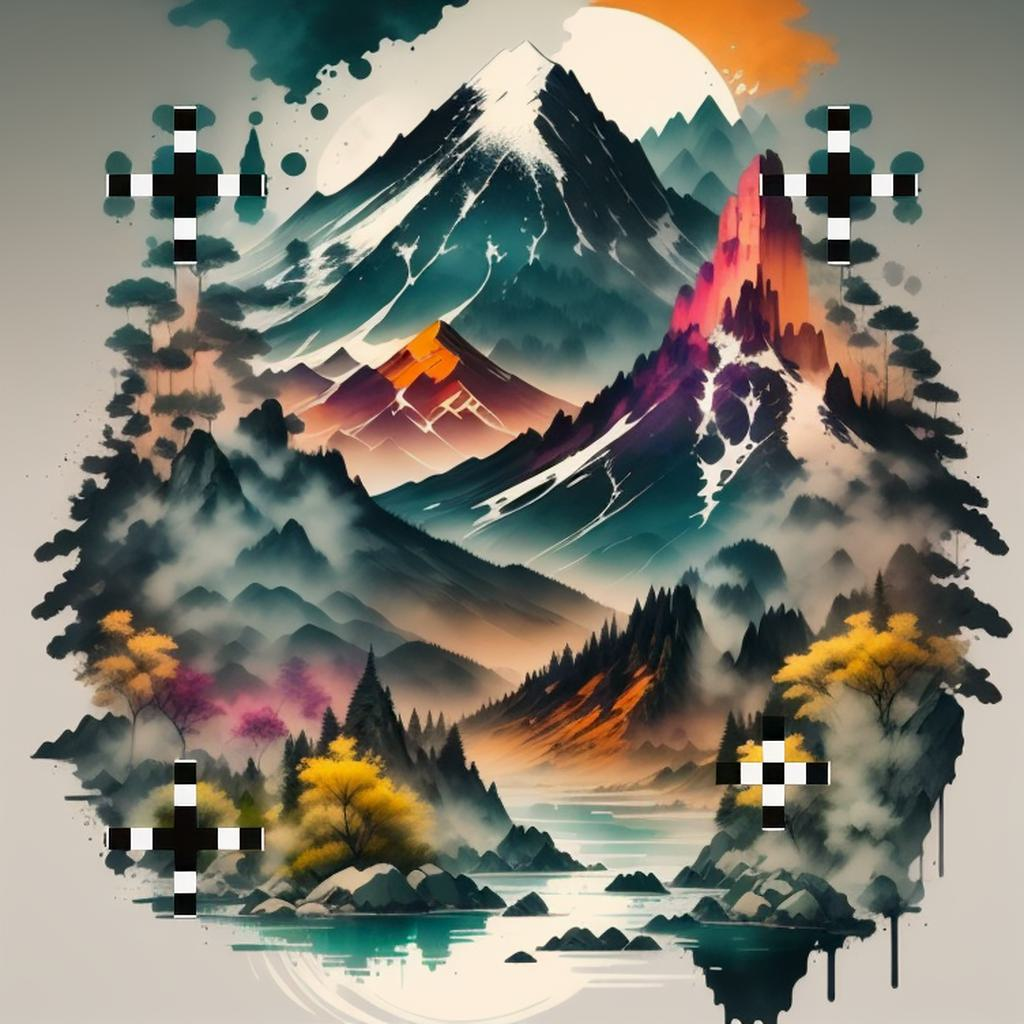} & 
    \includegraphics[width=\myfigwidth, height=\myfigwidth]{CVPR2024-T2QR/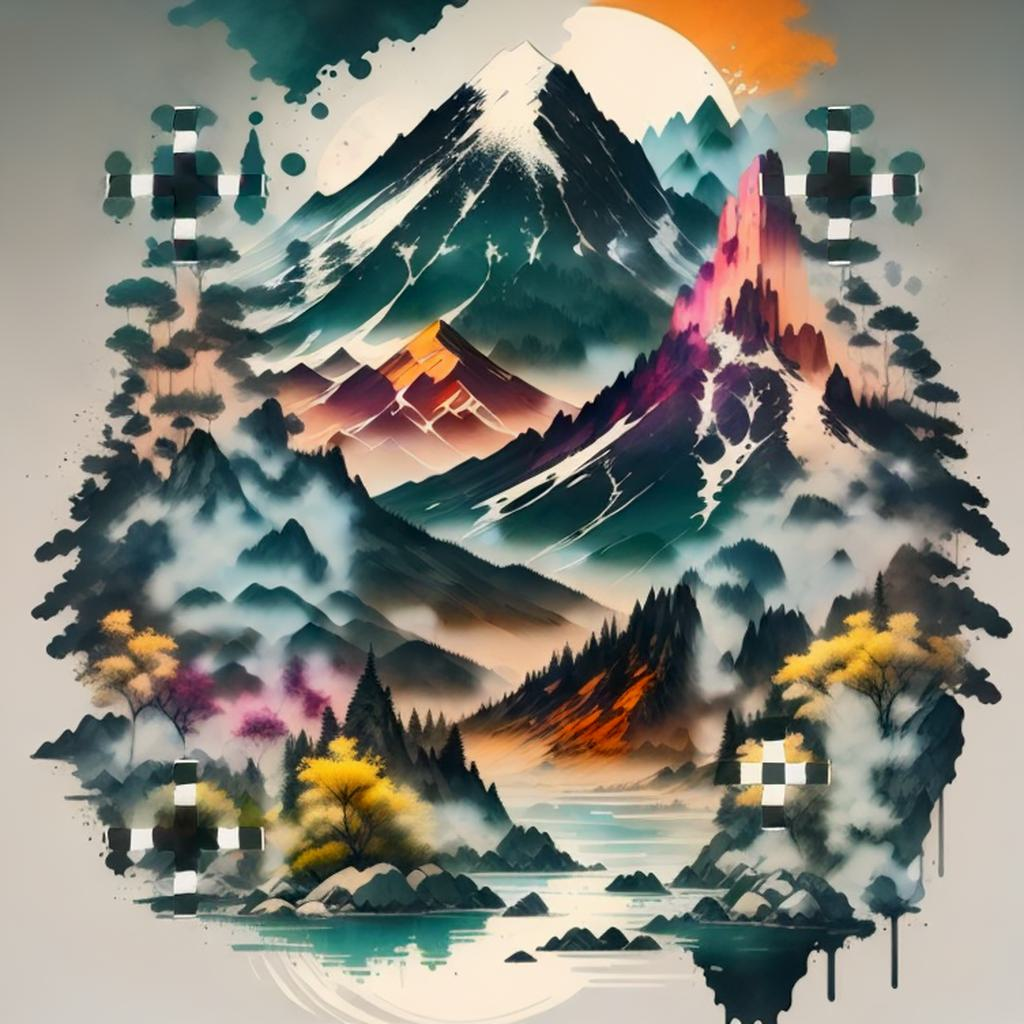} & 
    \includegraphics[width=\myfigwidth, height=\myfigwidth]{CVPR2024-T2QR/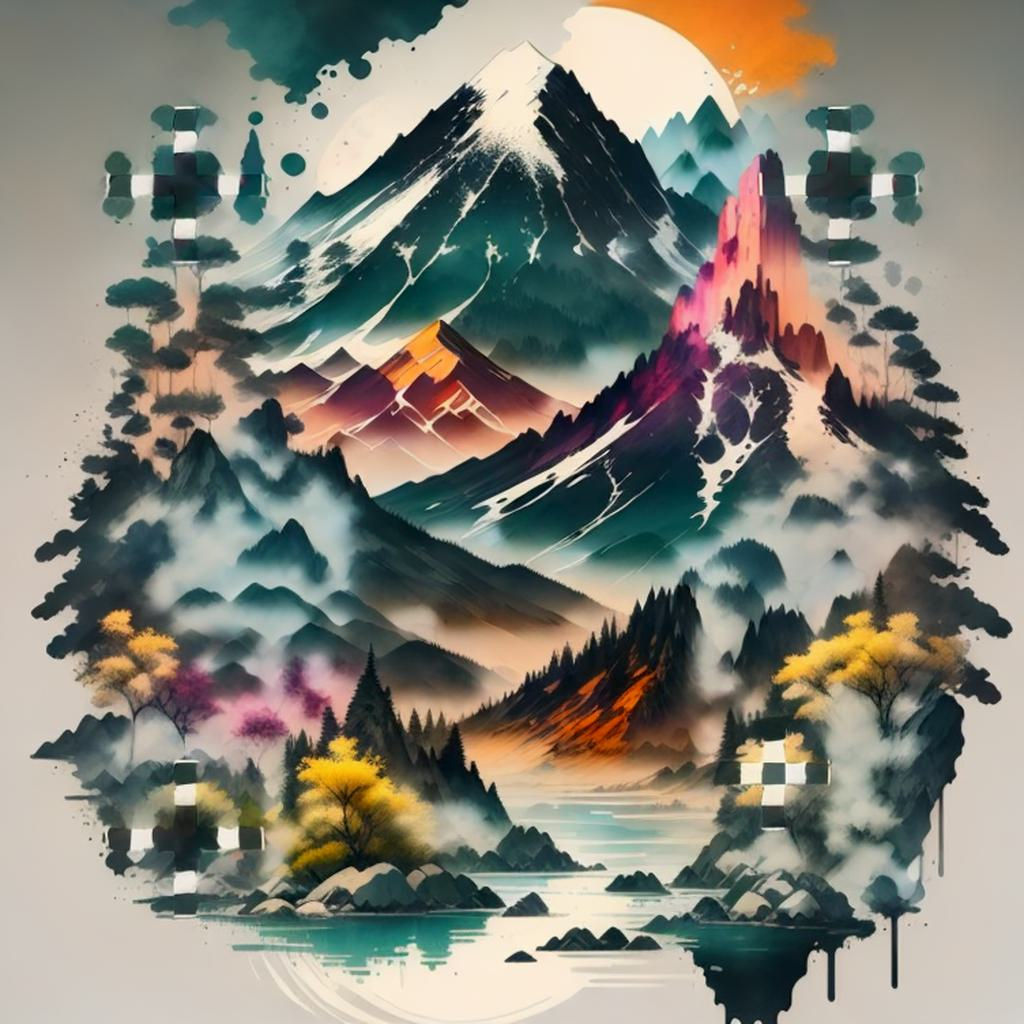} & 
    \includegraphics[width=\myfigwidth, height=\myfigwidth]{CVPR2024-T2QR/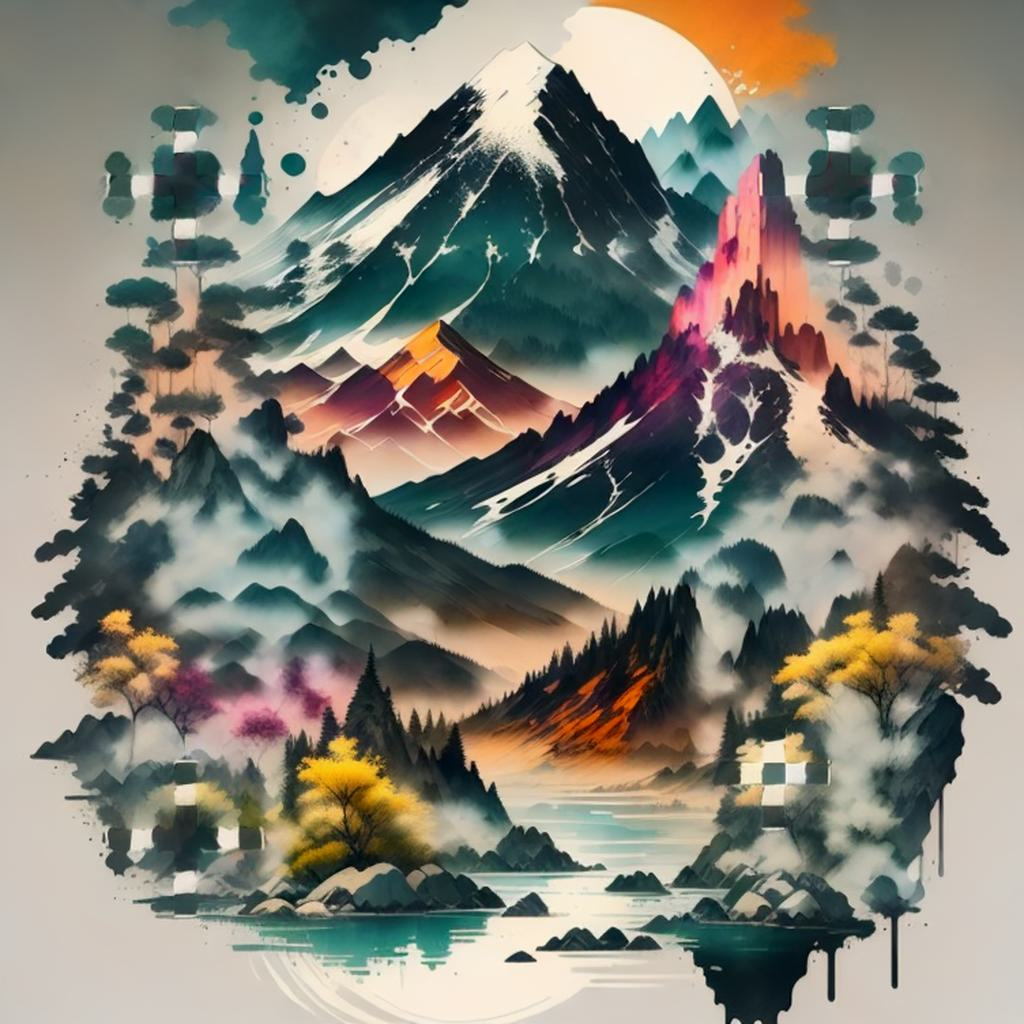} \\

    \includegraphics[width=\myfigwidth, height=\myfigwidth]{CVPR2024-T2QR/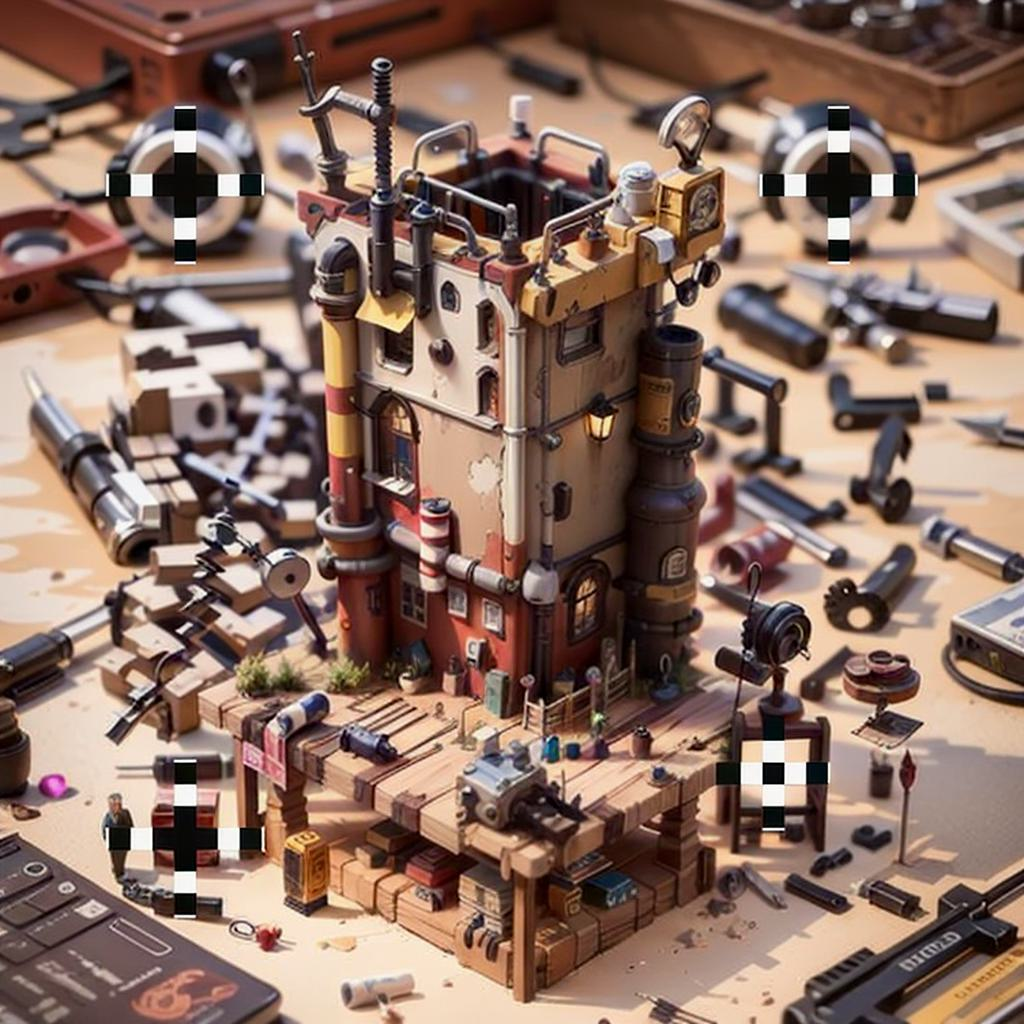} & 
    \includegraphics[width=\myfigwidth, height=\myfigwidth]{CVPR2024-T2QR/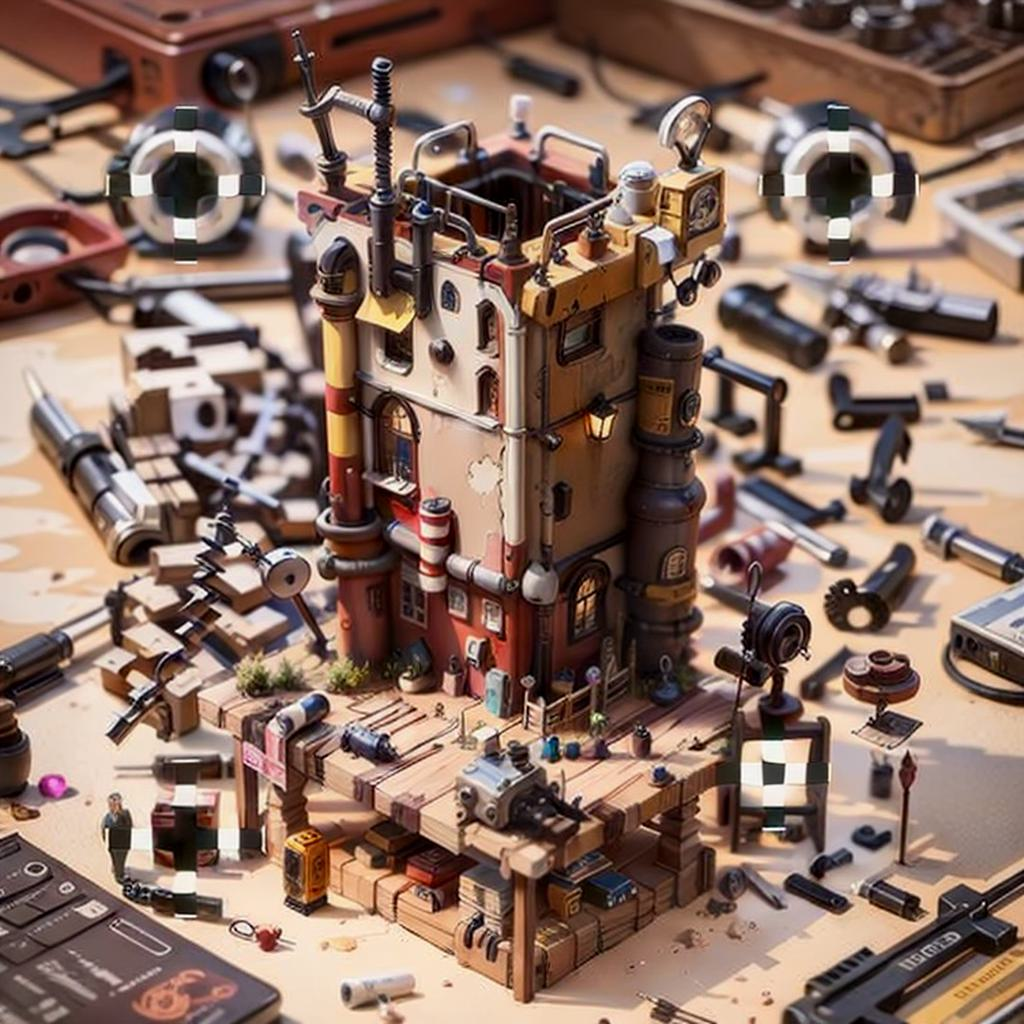} & 
    \includegraphics[width=\myfigwidth, height=\myfigwidth]{CVPR2024-T2QR/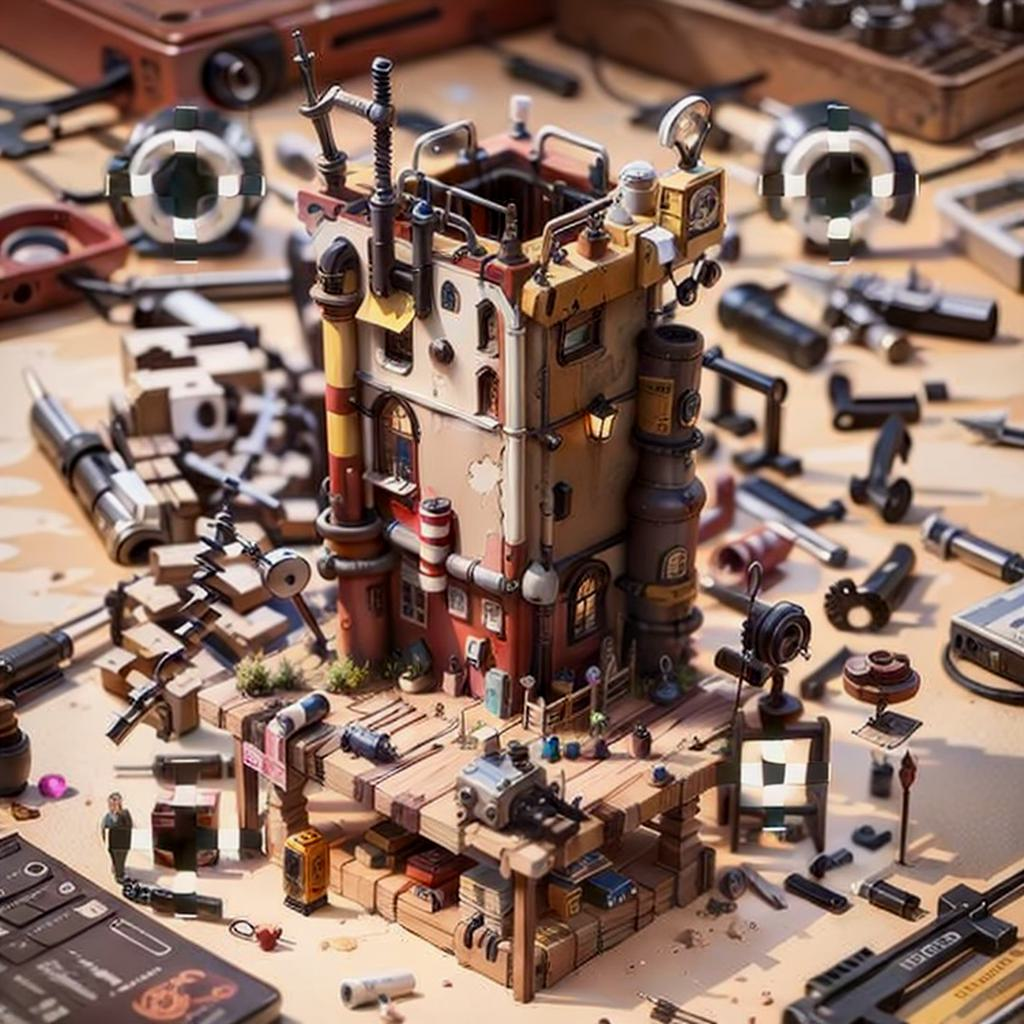} & 
    \includegraphics[width=\myfigwidth, height=\myfigwidth]{CVPR2024-T2QR/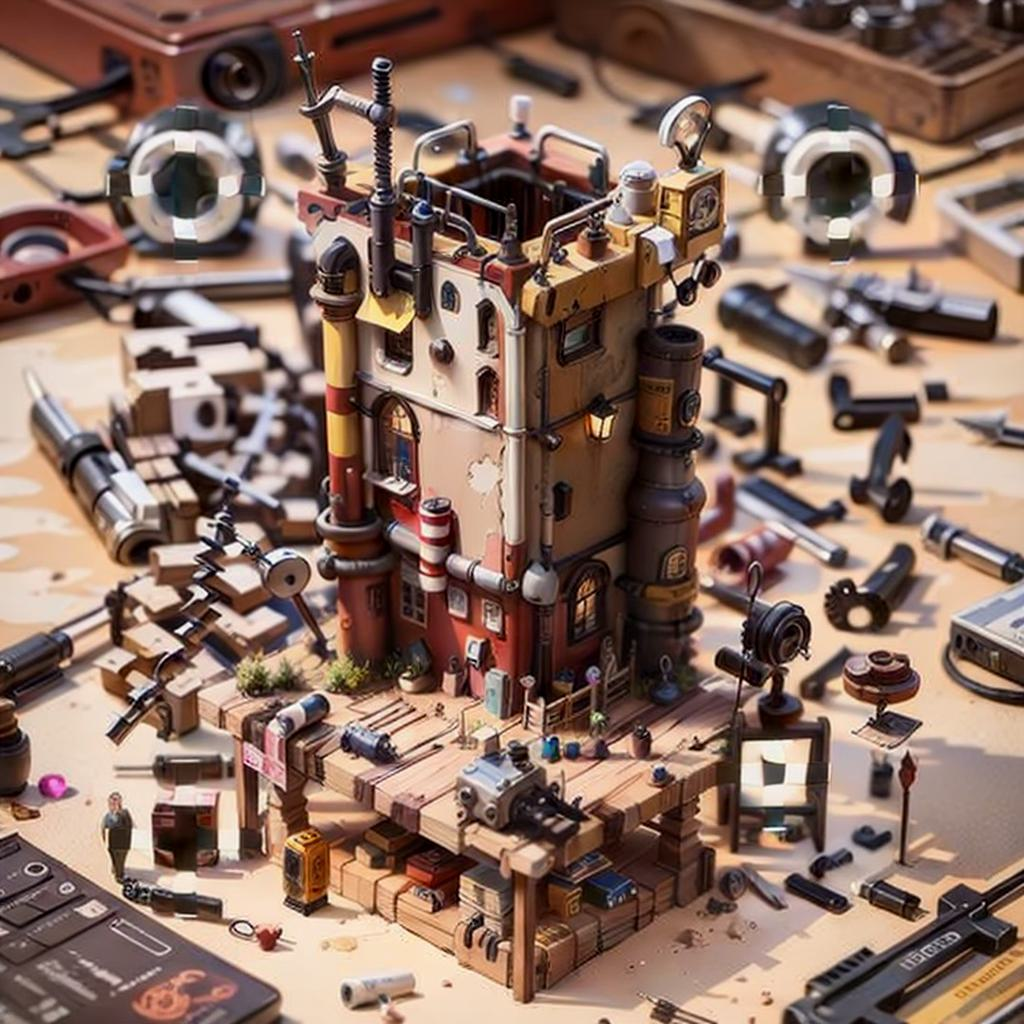} \\

    \bottomrule
    \end{tabularx}

\end{table}
    
Table~\ref{tab:selr} presents samples from various iterations in the SELR procedure. The iterative process seamlessly enhances the scanning robustness of the generated QR codes.

\section{Additional Visual Comparisons}
In Table~\ref{tab:comparison2}, we expand upon comparisons with prior methods. Additionally, Table~\ref{tab:comparison3} presents pertinent prompts and models associated with the generation of the aforementioned samples.

\section{Bad cases}
As shown in Figure~\ref{fig:bad}, we present suboptimal cases generated using a random prompt generator. Despite the less satisfying aesthetic quality, they still exhibit robust scanning robustness. The suboptimal cases arise from misalignments between prompt and model, a fundamental challenge in multi-modal large language models. Addressing this basic issue in future improvements will contribute to enhancing our overall performance.

\begin{figure}
    \centering
    \includegraphics{CVPR2024-T2QR/figs/rebuttal/bad-case.png}
    \caption{Bad cases derived from misalignments between prompt and model.}
    \label{fig:bad}
\end{figure}
\input{figs/suppl_1.tex}
\input{figs/suppl_2.tex}
\input{figs/suppl_3.tex}
